# Supplementary material for: Learning to Generalize Across Long-Horizon Tasks from Human Demonstrations
Source: arXiv:2003.06085 source file (2021-06-23)
Supplement: Supplementary file 1 [file 7_appendix.tex]

\section{Appendix}
\label{s_app}
